# Supplementary material for: Bias and high-dimensional adjustment in observational studies of peer effects
Source: arXiv:1706.04692 ancillary file (2017-06-14)
Supplement: Supplementary file 1 [file si.pdf]

# Supplementary Information for *Bias and high-dimensional adjustment in observational studies of peer effects*

## Contents

|          |                                                                              |           |
|----------|------------------------------------------------------------------------------|-----------|
| <b>1</b> | <b>Data</b>                                                                  | <b>2</b>  |
| 1.1      | Original experiment . . . . .                                                | 2         |
| 1.2      | Nonexperimental control group . . . . .                                      | 3         |
| <b>2</b> | <b>Methods</b>                                                               | <b>4</b>  |
| 2.1      | Number of strata per domain . . . . .                                        | 4         |
| 2.2      | Naive analysis . . . . .                                                     | 4         |
| 2.3      | Statistical inference . . . . .                                              | 6         |
| 2.4      | Illustration of distribution of estimated propensity scores . . . . .        | 7         |
| <b>3</b> | <b>Additional results</b>                                                    | <b>9</b>  |
| 3.1      | Comparisons of estimators . . . . .                                          | 9         |
| 3.2      | Maximum possible error . . . . .                                             | 10        |
| 3.3      | By prior popularity . . . . .                                                | 10        |
| 3.3.1    | Local regression of estimates on prior popularity . . . . .                  | 10        |
| <b>4</b> | <b>Explanations of observational–experimental discrepancies</b>              | <b>14</b> |
| 4.1      | Total peer effects versus peer effects of exposure for the exposed . . . . . | 14        |
| 4.2      | Individuating URLs . . . . .                                                 | 15        |
| <b>5</b> | <b>Evidence on bias and bias adjustment from prior DRPTs</b>                 | <b>16</b> |

# 1 Data

## 1.1 Original experiment

We analyze a large experiment that randomly modulated a primary mechanism of peer effects in information and media sharing behaviors. Bakshy et al. (2012) randomly assigned some user–URL pairs to a *no feed* condition: for pairs in that condition, those users would not see that URL in their Facebook News Feed. On the other hand, for user–URL pairs assigned to the *feed* (i.e., status quo) condition, those individuals can see that URL and associated comments by their peers; of course, if their peers do not share the URL, they still will not see it. Less than 1% of all user–URL pairs that would have resulted in exposure are assigned to the no feed condition. Even for pairs in the no feed condition, users could still see that their peer shared the URL if, e.g., the peer sent it to them in a message or posted it to the user’s profile. We refer readers to Bakshy et al. (2012) for further details about the experiment and other analyses of the experimental data.

This experiment identifies the average effect of exposure to peer URL sharing on Facebook for user–URL pairs for which that individual would have been exposed; this quantity can be described as the average treatment effect on the treated (ATT), for each treatment of exposure to one through six peers sharing the URL. We restrict our analysis to a single peer sharing the URL. More formally, for individuals who would have been exposed to a peer sharing a URL, the experiment identifies

$$\delta = \Pr(Y_{iu}(1) = 1 \mid E_{iu} = 1) - \Pr(Y_{iu}(0) = 1 \mid E_{iu} = 1) \quad (1)$$

$$= p^{(1)} - p^{(0)} \quad (2)$$

where  $E_{iu} = 1$  if and only if  $i$  would have been exposed to a peer sharing  $u$ ,  $Y_{iu} = 1$  if and only if  $i$  shares  $u$ , and  $Y_{iu}(1)$  and  $Y_{iu}(0)$  are the potential outcomes when exposed and when not exposed, respectively.<sup>1</sup>

We restrict our analysis to Facebook users believed to be located in the United States and using Facebook in American English and to domain names with at least 10,000 individual–URL pairs in the experimental data set.<sup>2</sup> This set of domains includes 3,704 with any prior sharing in our sample and 280 domains without prior sharing. This results in an experimental data set with 35 million users, 7.5 million URLs, and 74 million user–URL pairs exposed to a peer sharing the URL; this is the treated (exposed) group used in both the experimental and observational analyses. The experimental control group has 48 million users, 9.9 million URLs, and 147 million user–URL pairs.

---

<sup>1</sup> If one assumes that exposure via News Feed is the exhaustive, deterministic mechanism by which a peer sharing a URL on Facebook  $Z_{iu}$  affects whether the ego shares that behavior, then this experiment would also identify

$$\Pr(Y_{iu}(Z_{iu} = 1) = 1 \mid Z_{iu} = 1) - \Pr(Y_{iu}(Z_{iu} = 0) = 1 \mid Z_{iu} = 1)$$

because we always have  $E_{iu} = Z_{iu}$  and thus this is equal to (1). We can be sure that this assumption is not strictly true. Some individuals can fail to be exposed even when peers share a URL, so the relationship between  $Z$  and  $E$  is stochastic, rather than deterministic. There can also be other ways that peer sharing can affect ego sharing besides exposure; however, it may be the case that, especially for weak ties, exposure via News Feed is almost an exhaustive mechanism of peer effects in URL sharing.

<sup>2</sup>This is a subset of the data used by Bakshy et al. (2012), which included data for users from all countries and language settings.

## 1.2 Nonexperimental control group

We constructed a nonexperimental control group (NECG)<sup>3</sup> with approximately ten-times the number of user–URL pairs in the experimental data set.<sup>4</sup> The full NECG is constructed so as to have a similar marginal distribution of individuals and URLs as the exposed group. That is, URLs appear in the NECG a number of times proportional to how many times each appears in the experimental data set. To form user–URL pairs from this set of repeated URLs, individuals were then sampled with probability proportional to the number of times they appear in the experiment. In expectation, this procedure produces a NECG with users and URLs with the same marginal distribution of characteristics as the exposed group. Thus, the potential source of bias in the observational estimates is in the pairing of users and URLs, not, e.g., in marginal distribution of user characteristics.

We constructed a NECG to be approximately 10 times the size of the combined treated and experimental control group. We did this since subsequent analysis using propensity scores would result in substantially down-weighting many of these user–URL pairs. The full non-experimental control group includes 67 million users, 11 million URLs, and 677 million pairs.

---

<sup>3</sup>In the context of methods in which individual treated and control units are matched with each other, this is sometimes called a *reservoir*.

<sup>4</sup>This is approximate because, for computational reasons, the sampling method used waited until the final step to filter out pairs that were actually exposed.

## 2 Methods

The  $L_2$ -penalized logistic regressions were fit with LIBLINEAR (Fan et al., 2008), in which  $\lambda$  is specified by setting a parameter  $C$ , where  $\lambda = 1/2C$ .

### 2.1 Number of strata per domain

Rosenbaum and Rubin’s (1984) original presentation of stratification on estimated propensity scores illustrated the technique with  $J = 5$  strata defined by quintiles for an example data set with 1,515 observations, as have many applications since (cf. Lunceford et al., 2004). With a small number of strata, there can be substantial within-strata covariate imbalances that can be reduced by using a larger number of strata. If the number of strata does not increase with  $n$ , then propensity score stratification is not asymptotically consistent, even under conditional unconfoundedness, and exhibits greater bias than matching methods in simulation studies (Lunceford et al., 2004). Imbens (2004) suggests that asymptotically, there is little disadvantage to using a large number of strata, though we have not seen examples of this in the literature. For these reasons, we use a comparatively larger number of strata than is common.

Since all stratification is done by domain, we choose a variable number of strata per domain. For simplicity, the notation above works with a parameter  $J$  common to all domains. Fig. S1 displays estimates of  $p^{(0)}$  for different values of  $J$ . The estimates increase with  $J$ , thus decreasing error. This suggests that, especially with large data sets, forming strata from quintiles results in substantial remaining bias (cf. Lunceford et al., 2004), and this supports our choice to use many more strata. However, for the smaller domains,  $J = 1,000$  results in some strata having only exposed units; in the worse case, over 10% of domains have at least one such exposed-only stratum (Fig. S2). While it is primarily the domains with fewer observations that are affected (so this does not affect the overall results much), for analyses of the individual domain-specific results (i.e., by prior popularity), we want to avoid this. On the other hand, for the larger domains,  $J = 1,000$  still results in large enough strata that they could be divided even more granularly.

Thus, we also consider selecting a domain-specific  $J_d$  that is a function of the number of observations for that domain. In particular, we have set  $J_d = \lfloor an_{d1}^v \rfloor$ , where  $n_{d1}$  is the number of exposed user–URL pairs for domain  $d$  and  $v \in (0, 1)$  and  $a \in (0, \infty)$  are constants. This results in both a number of strata and a number of observations per stratum that increase with sample size. We produced estimates using three variations on this:

- $a = 3, v = 1/2$ ; that is,  $J_d = \lfloor 3\sqrt{n_{d1}} \rfloor$ ,
- $a = 4, v = 1/2$ ; that is,  $J_d = \lfloor 4\sqrt{n_{d1}} \rfloor$ ,
- $a = 1, v = 2/3$ ; that is,  $J_d = \lfloor n_{d1}^{(2/3)} \rfloor$ ,

which each result in less than 1,000 strata for the smaller domains and greater than 1,000 for the largest. Each of these variations produces estimates of  $p^{(0)}$  that are close to each other and close to the estimate when  $J = 1,000$ . The results in the main text use  $J_d = \lfloor 4\sqrt{n_{d1}} \rfloor$ , though none of our conclusions are substantially modified by using either of the three choices.

### 2.2 Naive analysis

For the sake of comparison, we also conduct a more basic analysis that does not utilize propensity scores or other adjustment. To estimate the probability of sharing for unexposed user–URL pairs,

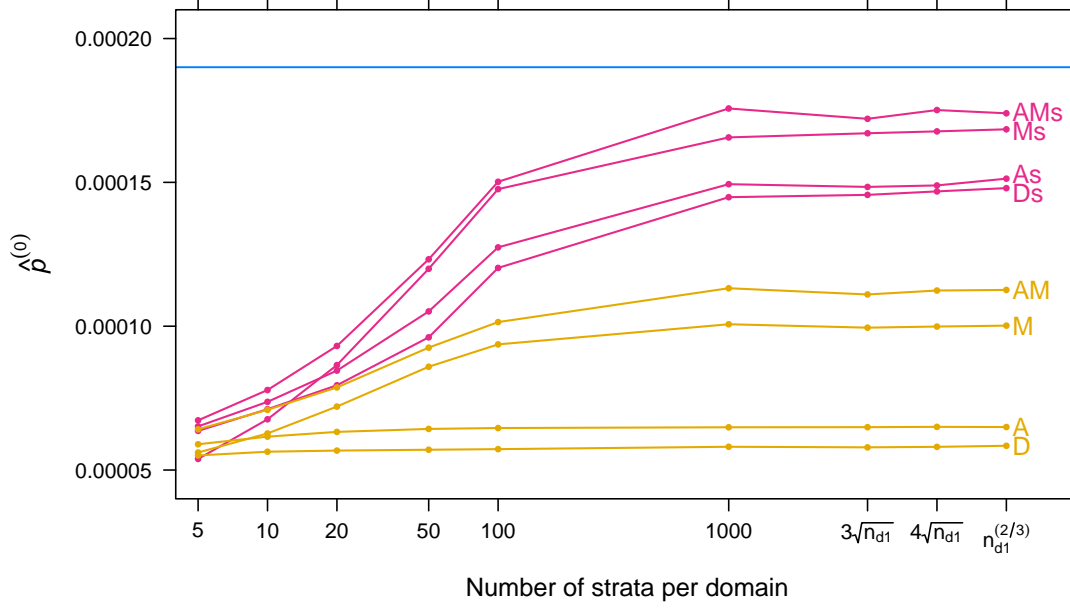

Figure S1: Estimates of  $p^{(0)}$  as a function of the number of strata  $J$  per domain. Increasing  $J$  results in larger estimates of  $p^{(0)}$ . The experimental estimate (blue) is greater than all of the displayed values, such that increasing  $J$  reduces estimated bias. The final three points superimposed on the  $x$ -axis correspond to estimators where the number of strata for a domain is a function of the number of treated units.

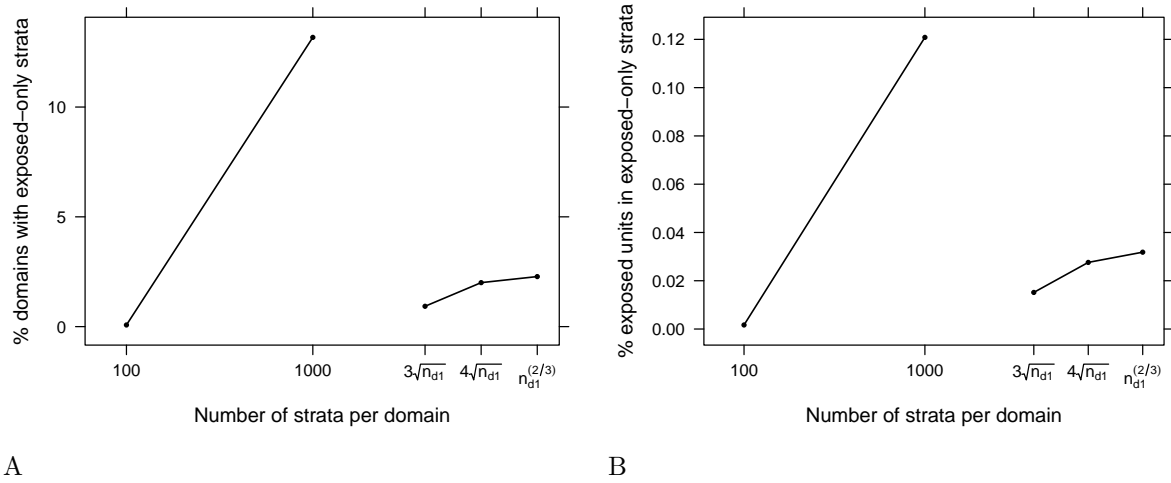

Figure S2: Missingness of strata as a function of the number of strata  $J$  per domain, illustrated for the full model (AMs). (A) Fraction of domains with at least one stratum containing only exposed units. For the case of a large fixed  $J$ , this is a substantial fraction of domains. (B) Fraction of exposed user-URL pairs in a stratum that does not contain control units. The domain-specific choices for  $J_d$  substantially reduce both of these measures by using a smaller number of strata from the domains with fewer observations.

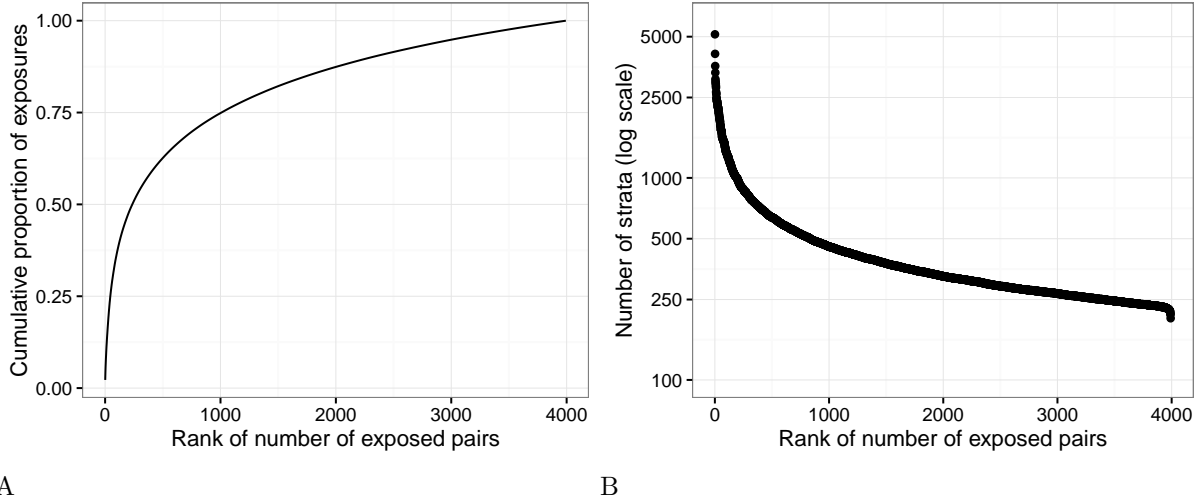

Figure S3: Distribution of exposures (A) and number of strata (B) per domain, sorted according to the number of observations (exposed user-URL pairs) for each domain. The number of strata in (B) is determined by  $J_d = \lfloor 4\sqrt{n_{d1}} \rfloor$ , which corresponds to the number of strata used to obtain the results in the main text and other sections of the supporting information.

we simply compute the proportion of user-URL pairs in the NECG that shared the URL for each domain. For analyses of multiple domains, we average these estimates, weighting each by the number of exposed user-URL pairs for that domain. Because the method by which the NECG was constructed approximated the marginal distribution of users from the exposed group, this approach can be seen as finding unexposed individuals similar to the exposed individuals, but without any adjustment for propensity to be exposed to different URLs. In the subsequent analysis, we refer to the resulting estimates as the *naïve observational estimates*.

## 2.3 Statistical inference

Our observations of both exposure and sharing are not independent and identically distributed (IID). Individuals vary in their probabilities of exposure and sharing, as do URLs. Exposure and sharing events are dependent, since an individual using Facebook at a particular time can often result in exposure to multiple URLs, and one person sharing a URL affects multiple others' exposure status. Methods for computing confidence intervals that neglect this dependence structure are expected to be substantially anti-conservative; that is, they would substantially overstate our confidence about the probability limit of each estimator.

To address this issue, all statistical inference in this paper employs a nonparametric bootstrap strategy for data with this crossed structure (Brennan et al., 1987; Owen, 2007; Owen and Eckles, 2012). For each of  $R = 100$  bootstrap replicates, we reweight observations according to the following procedure (Owen and Eckles, 2012). For the  $r$ th replicate, each individual is assigned a Bernoulli(0.5) draw, and each URL is assigned a binary random variable, a Bernoulli(0.5) draw. Each user-URL pair is then assigned the product of the corresponding draws as its weight. That is, a user-URL pair appears in a bootstrap replicate if and only if both the user and the URL are in the replicate. All procedures are applied to the original data set and each of the replicates, such that each propensity score model is fit  $R + 1 = 101$  times, quantiles of estimated propensity scores

for each domain are computed 101 times, etc. Under general conditions, this strategy is known to be conservative when estimating the variance of means (Owen, 2007; Owen and Eckles, 2012). Throughout, we report 95% bootstrap standard confidence intervals, which are expected to have at least 95% coverage due to variable-level duplication (Owen and Eckles, 2012). The bootstrap distribution of matching and resulting estimates is generally inconsistent because matching estimators do not satisfy required smoothness conditions for bootstrap validity, resulting in mildly incorrect confidence intervals (Abadie and Imbens, 2008). This is one motivation for using stratification, rather than one-to-one matching.

Note that all of the comparisons of interest are not entirely between-units. For example, the observational and experimental estimates share individuals, URLs, and (for comparing different observational estimates) even user–URL pairs. Observing that confidence intervals for two quantities overlap does not indicate that their difference (or ratio) is not statistically significantly different from zero (or one). This is one reason why we include figures showing estimates and intervals for relevant differences and ratios themselves. More specifically, many of the relevant comparisons are between different estimators computed on the same observations (e.g., comparisons of observational estimates of  $p^{(0)}$ , comparisons of error of observational estimates of  $RR$ ). Even observational–experimental comparisons involve common users and URLs.

## 2.4 Illustration of distribution of estimated propensity scores

Figure 1A in the main text displays the distribution of propensity scores for an example domain for the model **AMs**. Figure S4 displays these distributions of the other models. This illustrates that the models with smaller numbers of covariates yield much less dispersed estimated propensity scores in this example domain.

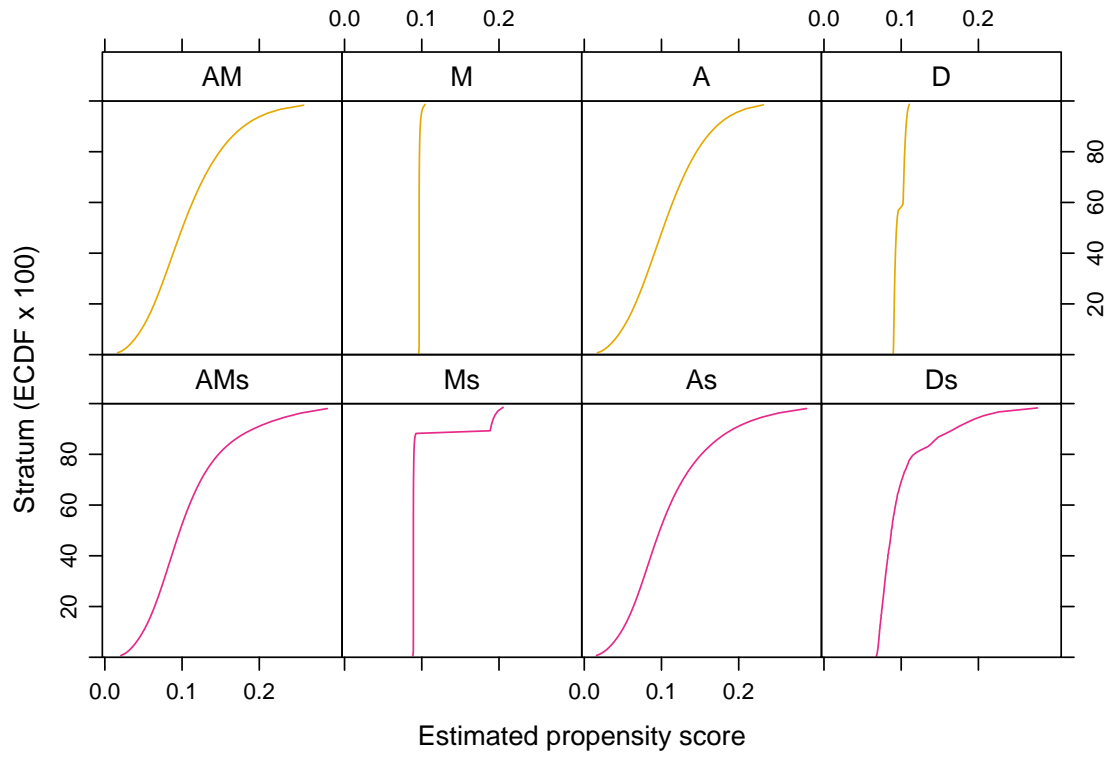

Figure S4: Observations are mapped to 100 strata (i.e., percentiles) based on the ECDF of the modeled propensity scores of exposed observations and unexposed observations in the NECG for [www.nytimes.com](http://www.nytimes.com). This expands the illustration in Figure 1A in the main text to compare multiple models.

Table S1: Tests comparing observational estimators. Each entry is the p-value for a  $\chi^2$  test that compares the estimated error in the relative risk. There are 28 tests, so the familywise error rate could be maintained at 0.05 by only rejecting the null when  $p < 1.79\text{e-}3$ .

|     | Ms      | AM      | M       | As      | Ds      | A       | D       |
|-----|---------|---------|---------|---------|---------|---------|---------|
| AMs | 3.1e-01 | < 1e-12 | < 1e-12 | 5.8e-04 | 4.0e-04 | < 1e-12 | < 1e-12 |
| Ms  |         | < 1e-12 | < 1e-12 | 4.9e-03 | 1.9e-03 | < 1e-12 | < 1e-12 |
| AM  |         |         | 1.2e-04 | 8.1e-07 | 1.3e-06 | < 1e-12 | < 1e-12 |
| M   |         |         |         | < 1e-12 | < 1e-12 | < 1e-12 | < 1e-12 |
| As  |         |         |         |         | 6.9e-01 | < 1e-12 | < 1e-12 |
| Ds  |         |         |         |         |         | < 1e-12 | < 1e-12 |
| A   |         |         |         |         |         |         | 1.2e-07 |

### 3 Additional results

#### 3.1 Comparisons of estimators

The observational estimates all arise from computing the corresponding estimator on the same data. For some pair of estimators, we can test the null hypothesis that they are estimating the same quantity using an asymptotic test for seemingly unrelated estimators. This is generalization of a Hausman specification test and is simply a  $\chi^2$  test. As with all statistical inference in the paper, we use the multi-way cluster robust bootstrap variance-covariance matrix. Table S1 displays the results of these tests for all estimators. Most of the comparisons are highly significant, though the pairs **AMs–Ms** and **As–Ds** are indistinguishable. After a conservative Bonferroni correction, the pairs **Ms–As** and **Ms–Ds** are indistinguishable.

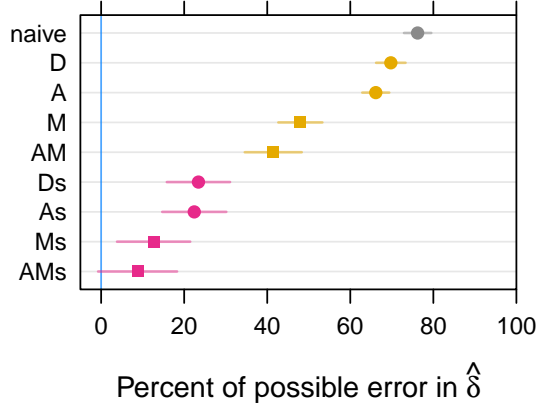

Figure S5: Estimated error in  $\hat{\delta}_m$  as a percent of the maximum possible overestimate arising from assuming  $p^{(0)} = 0$ . Error bars are 95% confidence intervals.

## 3.2 Maximum possible error

The main text characterizes the error of the naive and **AMs** estimators with respect to the maximum possible overestimate for  $\delta$ . Fig. S5 presents these results for all observational estimators.

## 3.3 By prior popularity

Fig. 3 in the main text shows estimated relative risk by quintiles of prior popularity. Fig. S6 we show the other quantities of interest by quintiles.

In the main text, we examine how bias and bias reduction for peer effects vary by the prior popularity of the domain of the URL. Here we present some additional summaries of these results, including statistical tests.

Many of the exposed user–URL pairs during the study are for URLs from domains that were very popular prior to the study (Spearman rank correlation = 0.43). Fig. S7 displays this relationship between prior popularity and number of exposed observations. The top 5% of domains by unique prior sharing users contribute 34% of exposed user–URL pairs.

We test the differences between each observational estimator and experimental estimator for each quintile of prior popularity (Fig. S8). This provides some formal statistical inferential support for the patterns noted in Fig. 3 in the main text.

### 3.3.1 Local regression of estimates on prior popularity

Fig. 3 in the main text and above show estimates by quintiles of prior popularity. Here we also include figures that do not require this discretization of prior popularity, but instead use local regression (loess).

We used loess to estimate expected  $p^{(0)}$  for all levels of prior popularity and model choice and  $p^{(1)}$  for all levels of prior popularity. This smoother was implemented using `loess` in R with a tricubic kernel. The width of the kernel was selected through the following cross-validation procedure applied to the fits to estimates of  $p^{(0)}$ . Domains were randomly partitioned into 10 folds. The model was fit to 10 subsets of the data, each leaving out one fold. Mean-squared error (MSE), weighted by the

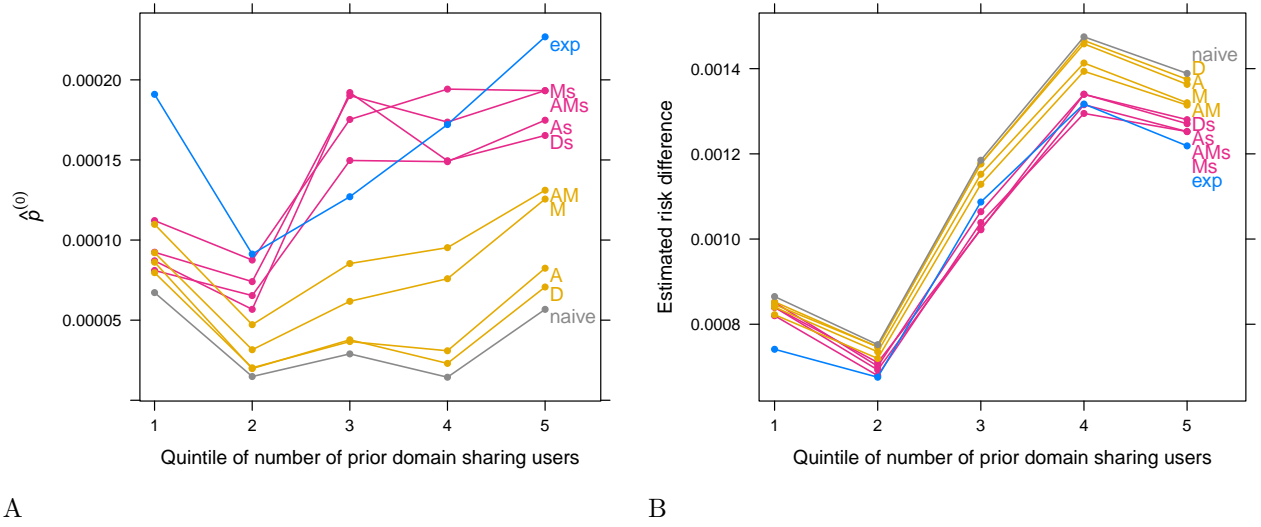

Figure S6: Estimates of (A)  $p^{(0)}$  and (B) risk difference for domains as a function of prior popularity, discretized by quintiles. Popularity is given in terms of quintiles of the number of unique users sharing URLs from the domain.

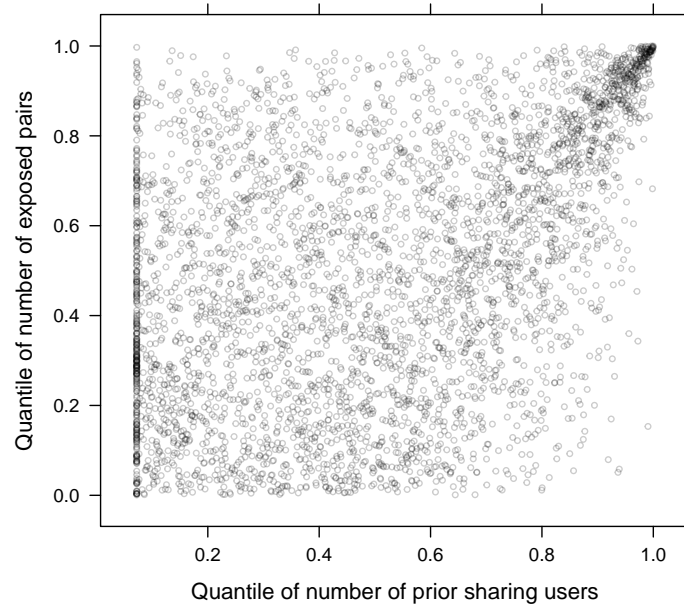

Figure S7: Association between the prior popularity of domains and the number of exposed user-URL pairs during the study.

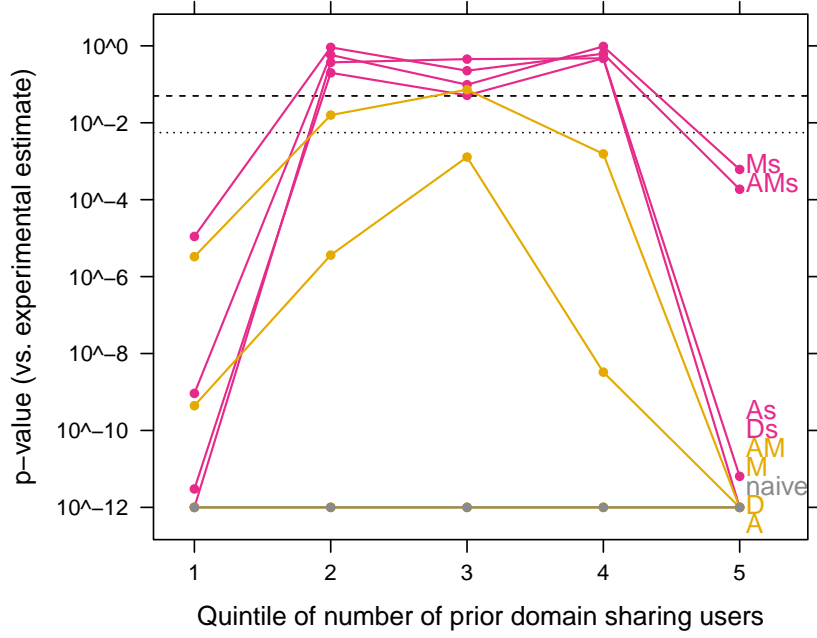

Figure S8: Tests comparing each of the observational estimators with the experimental one, by quintiles of prior popularity. Different thresholds for statistical significance are shown: 0.05 (black dashed line),  $0.05/(5 \times 9)$  for a familywise error rate of 0.05 (black dotted line).

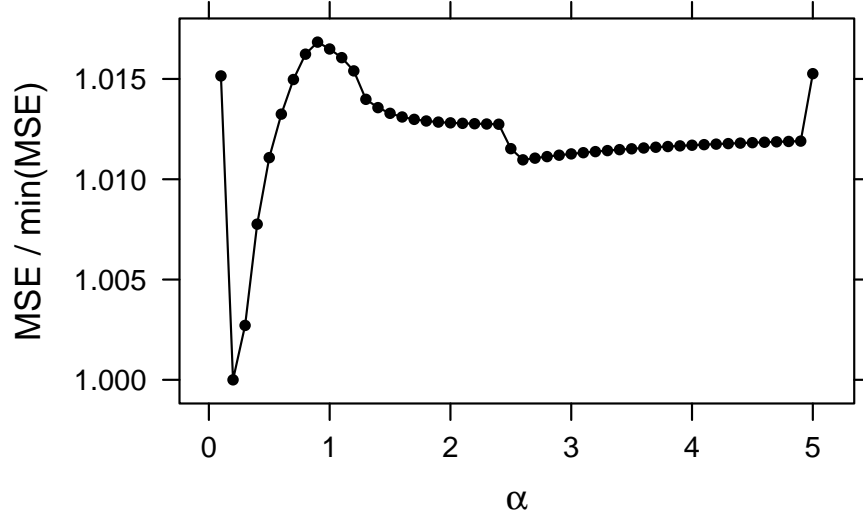

Figure S9: Mean-squared error in 10-fold cross-validation for model-specific, domain-specific estimates  $\hat{p}_{dm}^{(0)}$  averaged over all models.

number of exposed user–URL pairs, was computed for the out-of-sample domains for each value of the parameter  $\alpha \in \{0.1, 0.2, \dots, 5.0\}$ . The selected kernel width  $\alpha = 0.3$ , minimizes this weighted MSE averaged over all models (Fig. S9).

Fig. S10A displays the estimates of the probability of sharing when not exposed as a function of prior popularity. Domains that were more popular prior to the study have their URLs shared at higher rates even when users are not exposed to those URLs. One explanation of this is that users have other ways of discovering URLs from these popular sources. Fig. S10B and Fig. S10C repeats the analysis in terms of error in relative risk and maximum possible error in the risk difference by domain popularity.

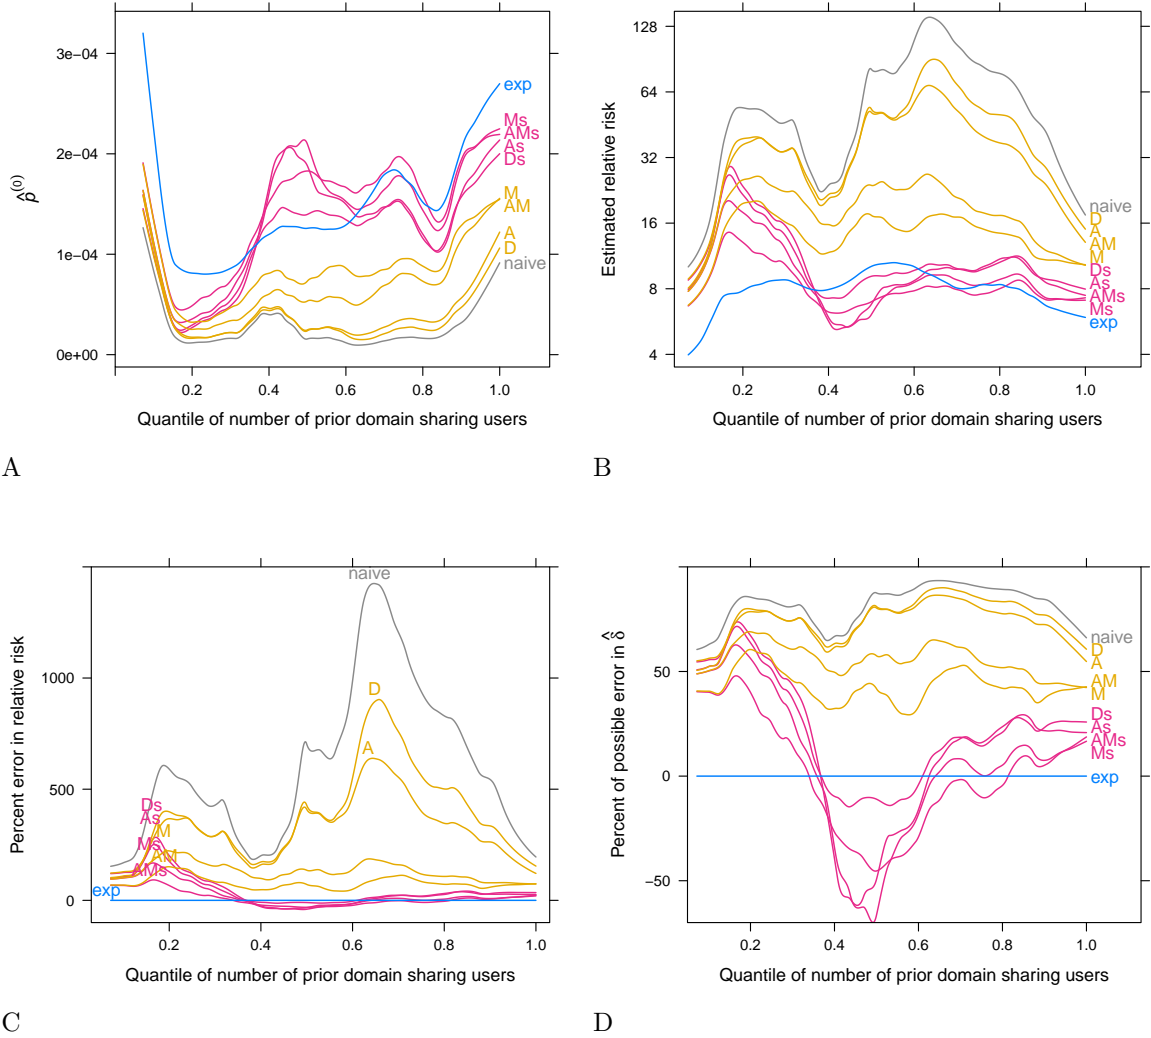

Figure S10: Observational estimators of  $p^{(0)}$  and their bias for domains as a function of prior popularity. We use local linear regression (loess) to combine domain-specific estimates of  $p^{(0)}$  and  $p^{(1)}$  that have similar prior popularity. Popularity is given in terms of quintiles of the number of unique users sharing URLs from the domain. Estimates of (A)  $p^{(0)}$  and (B) relative risk. (C) Estimated error in relative risk. (D) Estimated error in  $\delta_m$  as a percent of the maximum possible overestimate. Bandwidth of loess fit was determined by 10-fold cross validation (S2.6).

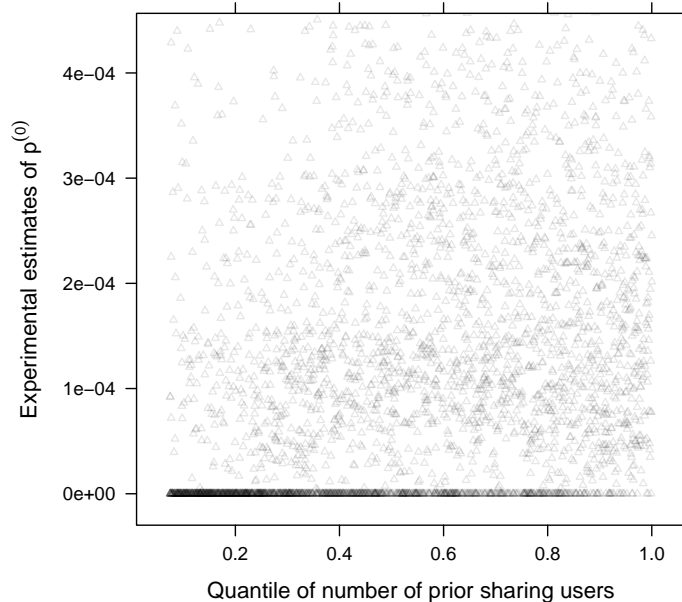

Figure S11: Experimental estimates of  $p^{(0)}$  by quantiles of the number of unique users sharing URLs from that domain in the prior six months. This further illustrates the variation in experimental estimates and that  $p^{(0)}$  is larger for the domains that are more popular prior to the study.

## 4 Explanations of observational–experimental discrepancies

We have regarded the experimental estimates as a “gold standard”. That is, we have regarded the experiment as identifying the average peer effects of interest for those who would be exposed. Thus, discrepancies between the experimental and observational estimates are then attributable to sampling variance in either and bias in the observational estimates. We expected the observational estimates to suffer from confounding bias because of selective tie formation and dissolution (i.e., homophily and heterophily), common external causes, and prior influence. Except for heterophily, these would all make it more likely for peers to share the same URLs, even in the absence of peer effects, so we anticipated that the naive observational analysis would overestimate peer effects, and that the estimators using propensity score stratification would reduce, but not eliminate or reverse, this bias. This is the primary explanation of differences between the the experimental and observational estimates. In this section, we consider two alternative explanations of differences between these estimates.

### 4.1 Total peer effects versus peer effects of exposure for the exposed

Even if total average peer effects are conditionally unconfounded given the covariates used in our propensity score models, the observational and experimental estimates can differ if the former consistently estimate total peer effects (i.e., effects of peer sharing via all mechanisms) and the latter consistently estimate peer effects of exposure through News Feed. This places an important limitation on what we can learn from this constructed observational study. We nonetheless regard studies such as this as one of the best available tools for better understanding the performance of observational methods for estimating peer effects.

We expect that while exposure via News Feed is not an exhaustive mechanism for peer effects in URL sharing on Facebook, it may be nearly exhaustive, since the other primary mechanism is exposure through that peer sharing the URL on Facebook and then, *because of this prior sharing decision*, sharing with the ego via some other method (e.g., via email, in person, or through Facebook private messaging). While sharing via other methods may be common, and this may be associated with sharing on Facebook, we expect that doing so as a result of having also done so on Facebook is relatively rare. We also note that Bakshy et al. (2012) find that, because weak ties are much more numerous than strong ties, most of the aggregate peer effects in URL sharing are caused by exposure to weak ties sharing as URL; for these weak ties, other communication is less likely.

## 4.2 Individuating URLs

One possible reason that the experimental estimates might not be a true (i.e. unbiased) “gold standard” concerns how URLs are individuated. The original experiment attempted to canonicalize URLs — that is, to identify multiple URLs that correspond to the same online resource and map them to the same canonical URL used for randomization and logging. However, there are some cases where this canonicalization is not sufficient. For example, there are sometimes variations on a URL (e.g., additions to the query “GET” parameters in the URL) that are designed to track how the user arrived at that URL.

For the purpose of studying peer effects in information diffusion, media consumption and sharing, etc., treating two URLs as distinct, such that an individual is only counted as sharing the same URL if they share a version that matches this appended set of query parameters exactly, is likely undesirable. Consider an individuals who would be exposed to a peer sharing a URL with the query parameters (i.e.,  $E_{iu} = 1$ ). They might encounter the same content through other means, in which case the URL would likely not have these parameters, or have different ones, and share that URL. Under the experimental analysis in Bakshy et al. (2012) and in this study, they would not be counted as sharing the URL. If we would prefer to consider these to be the same URL, then this results in underestimating  $p^{(0)}$  and  $p^{(1)}$  and likely overestimating their difference and ratio. One domain where this may be the case is `www.npr.org`.

## 5 Evidence on bias and bias adjustment from prior DRPTs

In the main text, we comment on prior papers that report on doubly-randomized preference trials (DRPTs). In particular, we note that the experimental comparison provides little-to-no formal statistical evidence; rather, any evidence about bias or bias reduction comes from comparisons *among* observational estimators, which are not actually reported in these papers, but can be partially inferred from the results reported.

First, the comparisons between observational and experimental estimators are not statistically significant. This can be determined by analysis of the reported point estimates and standard errors for the experimental and (unadjusted) observational data in Tables 2 and 3 of Steiner et al. (2010) and Table 3 of Pohl et al. (2009).<sup>5</sup>

Second, one can compare the different observational estimators. If there is evidence that two observational estimators (e.g., an unadjusted and adjusted) are converging to different estimands, then this might be interpreted as explained by the presence of confounding (though other explanations may be possible). In particular, using the reported point estimates and standard errors for various regression adjustment estimators (ANCOVA) in Tables 2 and 3 of Steiner et al. (2010), one can conduct Wu–Hausman specification tests of the null hypothesis that the different estimators estimate the same quantity. These tests are potentially anti-conservative for some of the estimators (e.g., the matching estimators) because of unknown covariance between the estimators (i.e. seemingly unrelated estimator tests should be used). We find that some of these tests (such as between the unadjusted and fully adjusted estimators) reject, which may be interpreted as providing entirely observational evidence for confounding. Thus, ironically, any statistical evidence for confounding bias or bias reduction through adjustment for covariates in Shadish et al. (2008) and Pohl et al. (2009) derives solely from the nonrandomized arms, not the randomized arms.

## References

- Abadie, A. and Imbens, G. W. (2008). On the failure of the bootstrap for matching estimators. *Econometrica*, 76(6):1537–1557.
- Bakshy, E., Rosenn, I., Marlow, C., and Adamic, L. (2012). The role of social networks in information diffusion. In *Proceedings of the 21st international conference on World Wide Web, WWW '12*, pages 519–528. ACM.
- Brennan, R. L., Harris, D. J., and Hanson, B. A. (1987). The bootstrap and other procedures for examining the variability of estimated variance components in testing contexts. Technical report, American College Testing Program.
- Fan, R.-E., Chang, K.-W., Hsieh, C.-J., Wang, X.-R., and Lin, C.-J. (2008). LIBLINEAR: A library for large linear classification. *The Journal of Machine Learning Research*, 9:1871–1874.
- Imbens, G. W. (2004). Nonparametric estimation of average treatment effects under exogeneity: A review. *Review of Economics and Statistics*, 86(1):4–29.
- Lunceford, J. K., Davidian, M., Lunceford, J. K., and Davidian, M. (2004). Stratification and weighting via the propensity score in estimation of causal treatment effects: A comparative study. *Statistics in Medicine*, 23(19):2937–2960.

---

<sup>5</sup>Note that Steiner et al. (2010) is a reanalysis of the data from Shadish et al. (2008), while Pohl et al. (2009) reports on an original study.

- Owen, A. B. (2007). The pigeonhole bootstrap. *The Annals of Applied Statistics*, 1(2):386–411.
- Owen, A. B. and Eckles, D. (2012). Bootstrapping data arrays of arbitrary order. *The Annals of Applied Statistics*, 6(3):895–927.
- Pohl, S., Steiner, P. M., Eisermann, J., Soellner, R., and Cook, T. D. (2009). Unbiased causal inference from an observational study: Results of a within-study comparison. *Educational Evaluation and Policy Analysis*, 31(4):463–479.
- Rosenbaum, P. R. and Rubin, D. B. (1984). Reducing bias in observational studies using subclassification on the propensity score. *Journal of the American Statistical Association*, 79(387):516–524.
- Shadish, W. R., Clark, H. H., and Steiner, P. M. (2008). Can nonrandomized experiments yield accurate answers? A randomized experiment comparing random and nonrandom assignments. *Journal of the American Statistical Association*, 103(484):1334–1344.
- Steiner, P. M., Cook, T. D., Shadish, W. R., and Clark, M. H. (2010). The importance of covariate selection in controlling for selection bias in observational studies. *Psychological Methods*, 15(3):250.
